# Supplementary material for: Image Transformer
Source: arXiv:1802.05751 source file (2018-06-15)
Supplement: Supplementary file 1 [file appendix.tex]

\section{CelebA Superresolution}

Image pairs comparing ratings of generated images by the Local 2D ImageTransformer model and the original images. On the left side are images where the raters prefer the generated image over the original ones. On the right side, raters prefer the original over generated image.

\begin{center}
\begin{longtable}[h!]{@{\hspace{.05cm}}c@{\hspace{.05cm}}c@{\hspace{1.5cm}}c@{\hspace{.05cm}}c} \\ 
 \endhead 
  \multicolumn{2}{c}{Local 2D $>$ Original} &  \multicolumn{2}{c}{Original $>$ Local 2D} \\
 Local 2D & Original & Local 2D & Original  \\
 {\includegraphics[width=.15\linewidth]{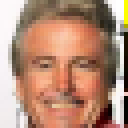}} 
 & {\includegraphics[width=.15\linewidth]{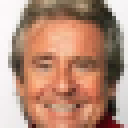}} 
 & {\includegraphics[width=.15\linewidth]{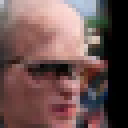}} 
 & {\includegraphics[width=.15\linewidth]{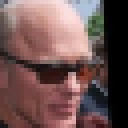}} 
  \\ [-0.75mm]
 {\includegraphics[width=.15\linewidth]{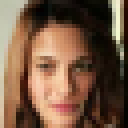}}
 & {\includegraphics[width=.15\linewidth]{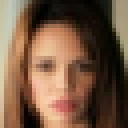}} 
 & {\includegraphics[width=.15\linewidth]{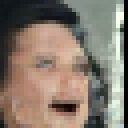}}
 & {\includegraphics[width=.15\linewidth]{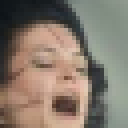}} 
 \\ [-0.75mm]
 {\includegraphics[width=.15\linewidth]{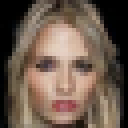}} 
 & {\includegraphics[width=.15\linewidth]{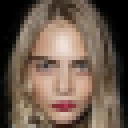}} 
 & {\includegraphics[width=.15\linewidth]{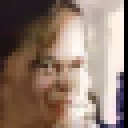}} 
 & {\includegraphics[width=.15\linewidth]{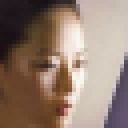}} 
 \\ [-0.75mm]
 {\includegraphics[width=.15\linewidth]{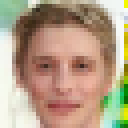}}
 & {\includegraphics[width=.15\linewidth]{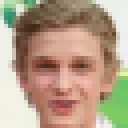}}
 & {\includegraphics[width=.15\linewidth]{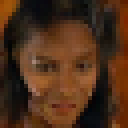}}
 & {\includegraphics[width=.15\linewidth]{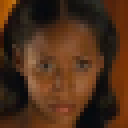}}
\\ [-0.75mm]

\end{longtable} 
\end{center}
